# Supplementary material for: ProJudge: A Multi-Modal Multi-Discipline Benchmark and Instruction-Tuning Dataset for MLLM-based Process Judges
Source: arXiv:2503.06553 source file (2025-03-09)
Supplement: Supplementary file 1 [file annotation_website.tex]

\begin{figure*}[!t]
\centering
  \resizebox{\linewidth}{!} {
    \includegraphics{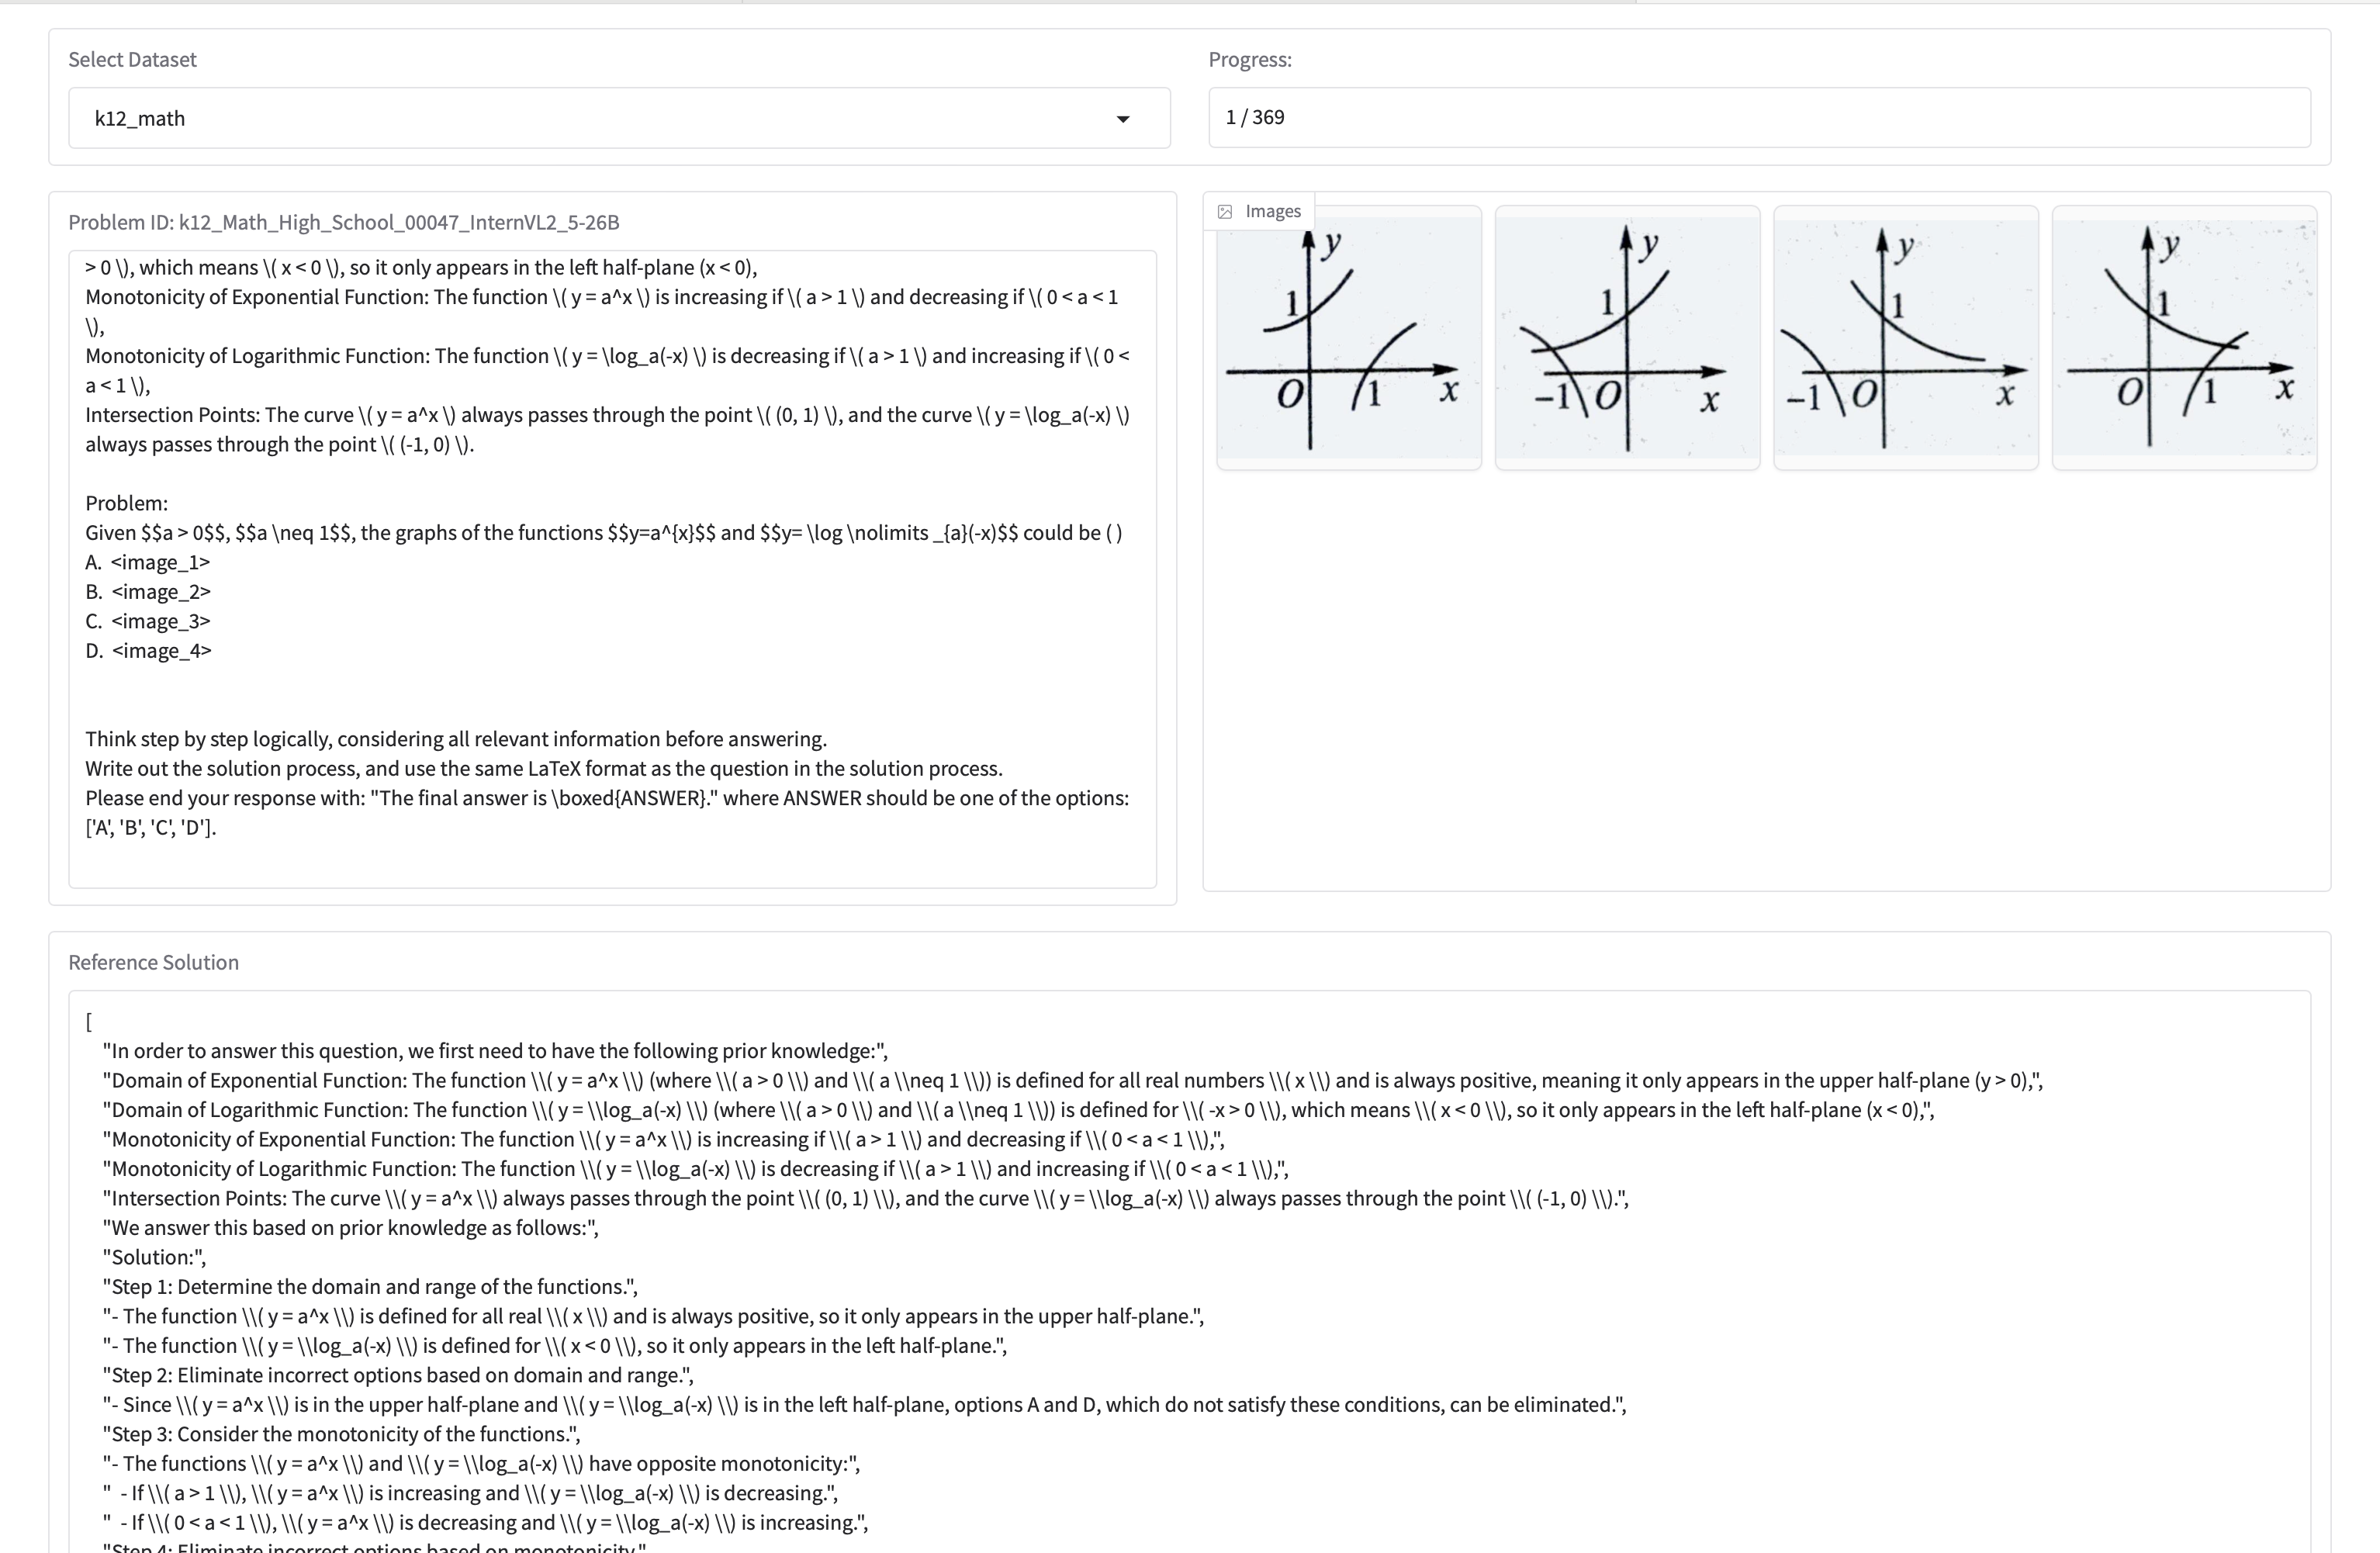}
  }
  \caption{Screenshot of annotation website.
  }
    \label{fig:annotation_website}
  \vspace{-5mm}
\end{figure*}
