# Supplementary material for: ProJudge: A Multi-Modal Multi-Discipline Benchmark and Instruction-Tuning Dataset for MLLM-based Process Judges
Source: arXiv:2503.06553 source file (2025-03-09)
Supplement: Supplementary file 2 [file 0_open_links.tex]

\section{Open-source Links}
All data and codes are available for viewing or download via the following URLs:

\begin{itemize}
    \item Project page: 
    \item GitHub repository:
    \item ProJudgeBench: 
    \item ProJudge-173k: 
\end{itemize}
